# Supplementary material for: Network Recasting: A Universal Method for Network Architecture Transformation
Source: arXiv:1809.05262 source file (2019-06-19)
Supplement: Supplementary file 1 [file yu_supp.pdf]

# A APPENDIX

## A.1 Activation Load

The input activations can be thrown away after convolution, but they should be fetched from the memory before the convolution. Thus the total amount of memory access for the activations is still the same as the total activation size. Also note that since the amount of output activations generated by the convolution is so big that they should be stored into the memory while they are generated. Therefore, stored activations have to be loaded at least once for convolution. For your info, state-of-the-art GPUs have only 3MB (Titan X Pascal) and 6MB (Tesla V100) L2 cache, but the smallest input activations per block of ResNet-50 and DenseNet-121 are 24.50MB and 6.13MB (with 64 batch size), respectively. Therefore, the output activations have to be stored in the off-chip memory.

## A.2 Details of ResNet and DenseNet

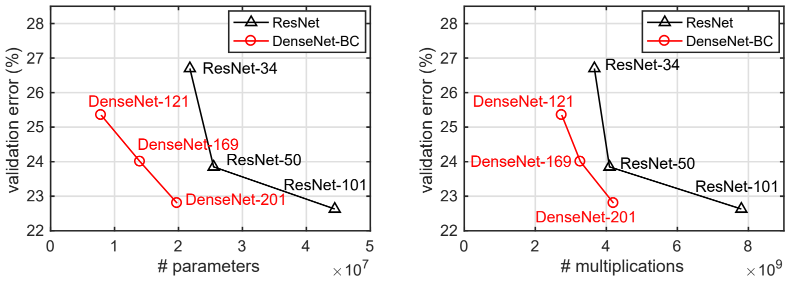


(a) The number of parameters (b) The number of multiplications

Figure 1: Comparison of parameters and multiplications between ResNet and DenseNet. We only count parameters and multiplication for convolution operation.

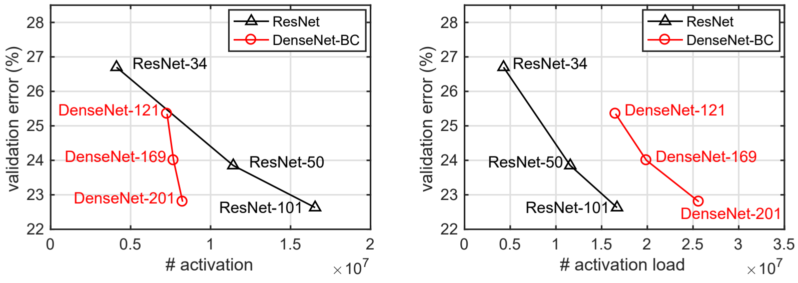


(a) Total activations size per image (b) Actual activation loads per image

Figure 2: Comparison of total number of activations and actual activation loads between ResNet and DenseNet. In DenseNet, following layers reuse output activations of all previous layers, so actual activation load is much larger than total activations. We count the number of activation elements for a single image.

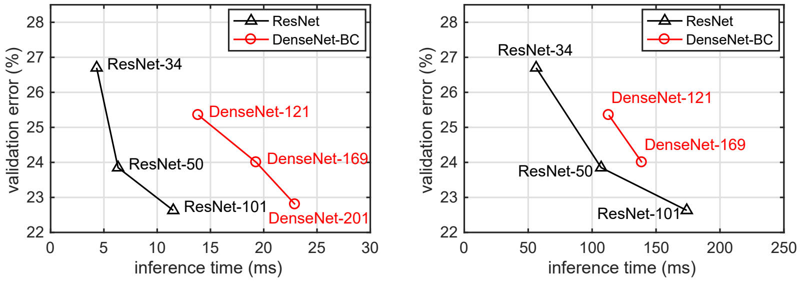


(a) Inference time (batch: 1) (b) Inference time (batch: 64)

Figure 3: Inference time for a single image and batch processing. When batch size is 64, DenseNet-201 cannot be run on an NVIDIA Titan X (Pascal) because it requires much more memory than GPU memory.

### A.3 Compression Example

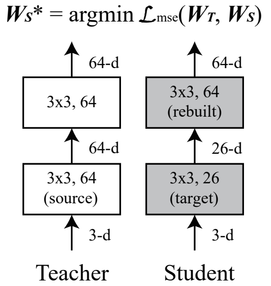


(a) VGG-16 compression

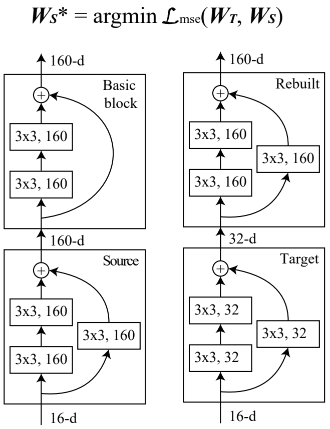


(b) WRN-28-10 compression

Figure 4: Examples of VGG-16 and WRN-28-10 compressions. Both example shows recasting of the first layer in each network.

Figure 4 illustrates the network compression process in VGG-16 and WRN-28-10. VGG-16 only has convolution block, so we recast the target block as smaller convolution block. As we mentioned Section 4.1, we recast every convolution block as $2.5\times$ smaller convolution block in VGG-16. In this reason, the number of filters is reduced from $64$ to $26$ in the recast block. To train the recast block, we use the next block and train both blocks by minimizing $\mathcal{L}_{mse}(W_T, W_S)$. After then, following blocks are recast and trained in the same manner.

WRN-28-10 is also compressed similar process to VGG-16 compression. We recast the target block as $5\times$ smaller basic block (from 160 to 32) as shown in Figure 4. Especially, we add new $1 \times 1$ convolution to the next block because of dimension mismatch. Both blocks are also trained to minimize $\mathcal{L}_{mse}(W_T, W_S)$. In next step, we also recast the next block as $5\times$ smaller basic block, but this recast block does not have $1 \times 1$ convolution because the dimension of input and output activation is the same with 32. Therefore, $1 \times 1$ convolution is added to train the recast block, and it is removed in next step. In this reason, there is no additional $1 \times 1$ convolution after sequential recasting.

### A.4 Description of Mixed Architectures

DenseNet-121 and ResNet-50 are recast as Recasting($R_{bs}$+D) and Recasting(C+$R_{bt}$) in ILSVRC2012 experiments, and Table 1 shows these mixed architectures. The round bracket ( ) indicates the convolutional layers with dense connection, and the square bracket [ ] denotes residual block. In addition, curly bracket { } means the convolution block. Every convolution has batch normalization and ReLU function.

Table 1: Mixed network Architectures for DenseNet-121 and ResNet-50

| Blocks | output size | DenseNet-121 | Recasting($R_{bs}$+D) | ResNet-50 | Recasting(C+$R_{bt}$) |
|---|---|---|---|---|---|
| conv1 | $112 \times 112$ | $7 \times 7$, 64, stride 2 | | | |
| pool1 | $56 \times 56$ | $3 \times 3$, max pool, stride 2 | | | |
| group1 | $56 \times 56$ | $\begin{pmatrix} 1 \times 1, 128 \\ 3 \times 3, 32 \end{pmatrix} \times 6$ | $\begin{bmatrix} 3 \times 3, 256 \\ 3 \times 3, 256 \end{bmatrix}$ | $\begin{bmatrix} 1 \times 1, 64 \\ 3 \times 3, 64 \\ 1 \times 1, 256 \end{bmatrix} \times 3$ | $\{3 \times 3, 64\} \times 3$ |
| Transition1 | $56 \times 56$ | $1 \times 1$, 128, stride 1 | | - | |
| | $28 \times 28$ | $2 \times 2$, average pool, stride 2 | | - | |
| group2 | $28 \times 28$ | $\begin{pmatrix} 1 \times 1, 128 \\ 3 \times 3, 32 \end{pmatrix} \times 12$ | $\begin{bmatrix} 3 \times 3, 512 \\ 3 \times 3, 512 \end{bmatrix}$ | $\begin{bmatrix} 1 \times 1, 128 \\ 3 \times 3, 128 \\ 1 \times 1, 512 \end{bmatrix} \times 4$ | $\{3 \times 3, 128\} \times 4$ |
| Transition2 | $28 \times 28$ | $1 \times 1$, 256, stride 1 | | - | |
| | $14 \times 14$ | $2 \times 2$, average pool, stride 2 | | - | |
| group3 | $14 \times 14$ | $\begin{pmatrix} 1 \times 1, 128 \\ 3 \times 3, 32 \end{pmatrix} \times 24$ | $\begin{pmatrix} 1 \times 1, 128 \\ 3 \times 3, 32 \end{pmatrix} \times 24$ | $\begin{bmatrix} 1 \times 1, 256 \\ 3 \times 3, 256 \\ 1 \times 1, 1024 \end{bmatrix} \times 6$ | $\{3 \times 3, 64\} \times 4$ <br> $\begin{bmatrix} 1 \times 1, 64 \\ 3 \times 3, 64 \\ 1 \times 1, 256 \end{bmatrix} \times 2$ |
| Transition3 | $14 \times 14$ | $1 \times 1$, 512, stride 1 | | - | |
| | $7 \times 7$ | $2 \times 2$, average pool, stride 2 | | - | |
| group4 | $7 \times 7$ | $\begin{pmatrix} 1 \times 1, 128 \\ 3 \times 3, 32 \end{pmatrix} \times 16$ | $\begin{pmatrix} 1 \times 1, 128 \\ 3 \times 3, 32 \end{pmatrix} \times 16$ | $\begin{bmatrix} 1 \times 1, 512 \\ 3 \times 3, 512 \\ 1 \times 1, 2048 \end{bmatrix} \times 3$ | $\begin{bmatrix} 1 \times 1, 512 \\ 3 \times 3, 512 \\ 1 \times 1, 2048 \end{bmatrix} \times 3$ |
| Classifier | $1 \times 1$ | $7 \times 7$, average pool, 1000-d FC, softmax | | | |

### A.5 Information on Tensor Core

For the experiments, we use NVIDIA Titan X (Pascal) and DGX-1 (It has eight Tesla V100 GPU). V100 has many Tensor Cores and those accelerate neural network training with low precision multiplication. However, this low precision multipliers make our proposed method diverged. After turning off Tensor Core during training time, we obtained correct results on NVIDIA Tesla V100. In this reason,we recommend turning off the Tensor Core when you want to use our proposed method.
